# Supplementary material for: Point defect states emergence in a plasmonic crystal
Source: arXiv:1908.11644 ancillary file (2019-08-30)
Supplement: Supplementary file 1 [file SM_PlasmonicCrystals.pdf]

# SUPPLEMENTAL MATERIAL

# Point defect state emergence in a plasmonic crystal

Hikaru Saito[1,*], Hugo Lourenço-Martins[2], Noémie Bonnet[2], Xiaoyan Li[2], Tracy C. Lovejoy[3], Niklas Dellby[3], Odile Stéphan[2], Mathieu Kociak[2], Luiz Henrique Galvão Tizei[2]

[1] Department of Advanced Materials Science and Engineering, Kyushu University, 6-1 Kasugakoen, Kasuga, Fukuoka 816-8580, Japan
[2] Laboratoire de Physique des Solides, Université Paris-Sud, CNRS-UMR 8502, Orsay 91405, France
[3] Nion Company, 1102 Eighth Street, Kirkland, Washington 98033, USA.

*corresponding author

**e-mail address**
saito.hikaru.961@m.kyushu-u.ac.jp

**Corresponding author's phone number, fax number**
Phone: +81-92-583-7579
Fax: +81-92-583-7580

**A. Plasmonic band structure under empty lattice approximation**

The dispersion relation calculated for the Al(50 nm)/$Si_3N_4$(15 nm) bilayer film with no structure is shown in Fig. S1a, which is expected to give the slope of the band dispersion under the empty lattice approximation (ELA). Here, the dielectric function for aluminum was derived by fitting the Drude-Lorentz model to the permittivity data given by Palik [S1]. The dielectric function for $Si_3N_4$ was set to the constant value 4 [S2]. The plotted two curves correspond to two SPP modes propagating along the top surface of the aluminum film and the bottom Al/ $Si_3N_4$ interface. The aluminum disk array is supposed to make large modification only in the dispersion relation of the top surface mode. We focused on the modified top surface mode although it is inevitable that information about the unstructured Al/Si3N4 interface are included as background intensity. The band dispersion of the SPP Bloch modes at the top structured surface was calculated under the ELA, as shown in Fig. 1b. The corresponding energy values of the SPP modes at the M and K points were calculated to be 1.79 eV and 2.04 eV, respectively.

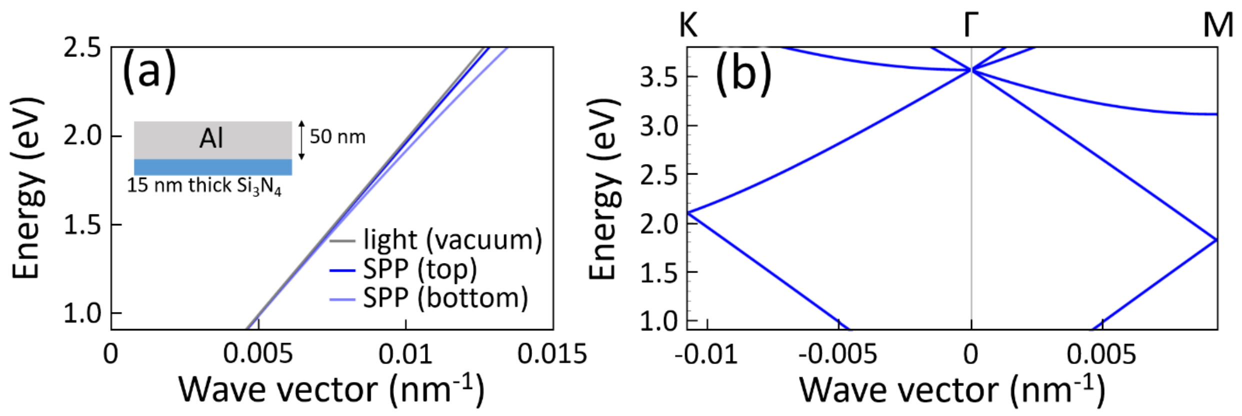


FIG. S1 (a) Theoretical dispersion relations of SPPs on the top surface and the bottom interface in the flat Al(50 nm)/ $Si_3N_4$(15 nm) double layer structure. (b) Theoretical plasmonic band structure under the ELA.

## B. FDTD simulation

FDTD simulation was performed using the CrystalWave software package (Photon Design) to calculate the field distribution of the band edge modes and the defect mode, and the dispersion relation of the five branches leading to the band edges.

### *B-1. Band edge modes at the M and K points*

Fig. S2 shows the distribution of normal electric component for each band edge modes $E_{z,l}(\mathbf{r})$ at the M and K points. The index *l* specifies the mode. The upper band edge mode at the K point is doubly degenerate. In Figs. 1d-1g (main text) the electric field strength after averaging based on the translational and the rotational symmetries are shown for each mode, which agree with the filtered maps from EELS spectrum images shown in Figs. 1b and 1c (main text). Regarding experimental filtered maps, the displayed intensity includes not only surface losses but also volume losses. In fact, over the whole energy range, the intensity in the blue and red spectra is higher than that in the green spectrum (Fig. 1a in the main text) because of the large difference in thickness. Therefore, the intensity only on the disks is displayed in Figs. 1b and 1c, where the contrast can be related to the surface normal component of electromagnetic local density of states (EMLDOS) [S3]. The intensity only on the outside the disks is shown in Fig. 1i for the same reason.

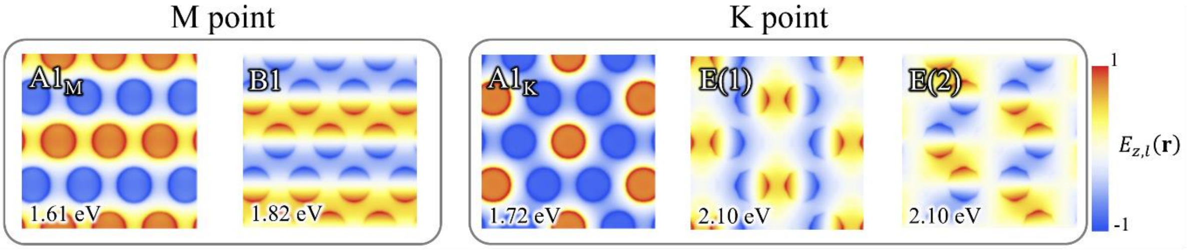


FIG. S2 $E_{z,l}(\mathbf{r})$ calculated at the M and K points by FDTD simulation.

Details for the calculation were described in the literature [S4]. Briefly, the calculation space was set to 784 nm × 680 nm × 2000 nm for $A1_M$ and B1 modes, and 1176 nm × 1360 nm × 2000 nm for $A1_K$ and E modes. The spaces were divided by cubic calculation voxels of 4 nm × 4 nm × 4 nm. The

sample was placed at the center of calculation space and surrounded by vacuum. The periodic boundaries were set at the end planes in the parallel directions to the sample surface. The perfectly matched layers (PMLs) were set at the end planes in the surface normal. The dielectric function for aluminum was derived by fitting the Drude Lorentz model to the permittivity data given by Palik [S1]. The dielectric function for $Si_3N_4$ was set to the constant value 4 [S2]. For the model structure in the FDTD simulation, an aluminum disk array with 260 nm diameter, 60 nm height and 392 nm period was placed on a flat aluminum (52 nm thick)/$Si_3N_4$ (16 nm) double layer film. The band edge modes were excited by point dipole oscillators positioned at the antinodes 100 nm above the disks' surface. The displayed field (Fig. S2) and field strength maps (Figs. 1d-1g in the main text) were extracted from the plane 8 nm above the top surface of the disks. Temporal change of electric field was Fourier transformed to obtain each spectrum.

***B-2. Defect mode***

Surface normal component of electric field strength (Fig. 1j in the main text) and spectra (Fig. 3e in the main text) of the point defect mode were calculated in the same way as above. However, we can not use periodic boundaries for the confined defect mode. A large calculation space (20000 nm × 20000 nm × 2000 nm) was set. The space was divided by cubic calculation voxels of 6 nm × 6 nm × 6 nm. For the model structure in the FDTD simulation, an aluminum disk array with 260 nm diameter, 42 nm height and 392 nm period was placed on a flat $Si_3N_4$ (18 nm) double layer film. The disks were covered by 54 nm-height silver layer just like the inset picture above Fig. 3a (main text). The defect mode was excited by a point dipole oscillator positioned at the center of defect 100 nm above the disk top. The temporal pulse width of the dipole exciters was set to 5 fs. The displayed field strength map (Fig. 1j in the main text) was extracted from the plane 8 nm above the top surface of the disks. Temporal change of electric field was Fourier transformed to obtain the spectrum (Fig. 3e in the main text). The time duration for the Fourier transformation was 42 fs, which starts 3 fs after finishing oscillation of the excitation dipole.

***B-3. Dispersion relations of five branches leading to the M and K points***

The five branches around the M and K point described in Fig. S3a were calculated in the same way as above. The calculation space in the parallel directions to the sample surface was adjusted so that a given mode satisfies the periodic boundary condition determined by its sides $L_M$ and $L_K$ (Fig. S3b), where $L_M$ and $L_K$ are integer multiples of the sides of unit cell a and b. A dipole oscillator array was placed in the period corresponding to the given modal wavelength so that it was selectively excited.

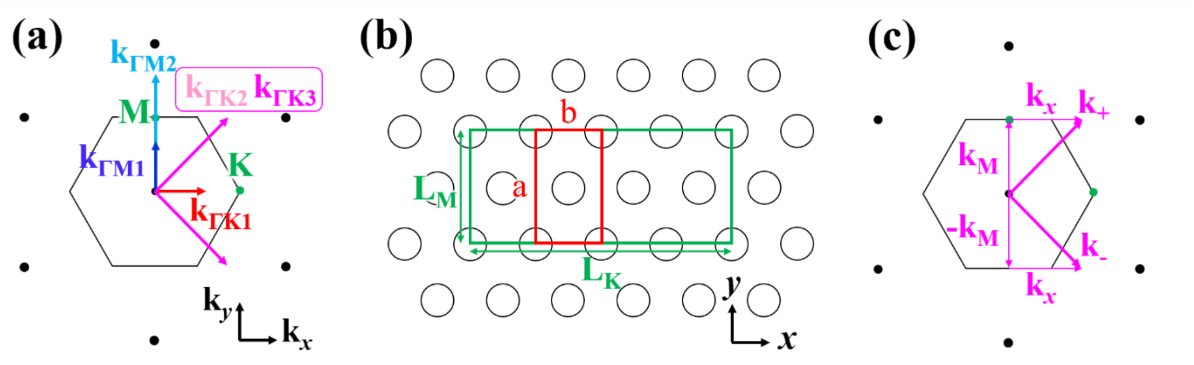


FIG. S3 (a) Schematic drawing of the reciprocal lattice for the triangular lattice and the five branches leading to the M and K points. (b) The calculation space in the parallel directions to the sample surface. (c) Two wave vectors $\mathbf{k}_+$ and $\mathbf{k}_-$ of the basis plane waves for the $\mathbf{k}_{\Gamma K2}$ and $\mathbf{k}_{\Gamma K3}$ modes and decomposition into $\mathbf{k}_M$ and $\mathbf{k}_x$.

From the K point to the Γ point in the second band, there are two basis plane waves with $\mathbf{k}_+$ and $\mathbf{k}_-$ (S3c) which are converted to each other by Bragg reflection in the surface. The two eigen modes $\mathbf{k}_{\Gamma K2}$ and $\mathbf{k}_{\Gamma K3}$ are described as linear combinations of the basis plane waves as follows using $\mathbf{k}_M$ and $\mathbf{k}_x$ under the ELA,

$$E_{z,\Gamma K2}(\mathbf{r}):\ e^{i(k_M y+k_x x)}+e^{i(-k_M y+k_x x)} \propto \cos k_M y\cdot e^{ik_x x} \quad \text{(S1)}$$

$$E_{z,\Gamma K3}(\mathbf{r}):\ e^{i(k_M y+k_x x)}-e^{i(-k_M y+k_x x)} \propto \sin k_M y\cdot e^{ik_x x} \quad \text{(S2)}$$

where terms expressing time and *z* dependence are omitted. The $\mathbf{k}_{\Gamma K2}$ mode is symmetric with respect to the center lines of the disk columns along the Γ-K direction and the antinodes are located at the Γ-K disk columns while the $\mathbf{k}_{\Gamma K3}$ mode is anti-symmetric with respect to the center lines and the antinodes are located between the Γ-K disk columns. For the $\mathbf{k}_{\Gamma K2}$ mode, the dipole oscillator array

was placed on the Γ-K disk columns while it was placed between the Γ-K disk columns for the $\mathbf{k}_{\Gamma K3}$ mode.

Upper branches $\mathbf{k}_{\Gamma M2}$, $\mathbf{k}_{\Gamma K2}$ and $\mathbf{k}_{\Gamma K3}$ enter partially above the light line due to Bragg reflection, resulting in low quality factors due to radiative loss. Peak broadening becomes severer with disk height *h* as shown in emission spectra calculated for the $\mathbf{k}_{\Gamma M2}$ mode with 0.0121 $nm^{-1}$ of wave number (Fig. S4). For *h* = 60 nm, the peak position can be clearly determined. However, for *h* = 96 nm, the peak position becomes ambiguous although a shoulder was observed in the lower energy side. Thus, the dispersion relation of the upper branches for *h* = 96 nm is not plotted in Fig. 2d (main text). Another strange peak appears at about 2.5 eV, which is above the corresponding photon energy 2.38 eV, meaning that is not an SPP mode. Such a strange peak above the light line was also observed in momentum-resolved CL experiments when the dark modes got closer to the light line [S5].

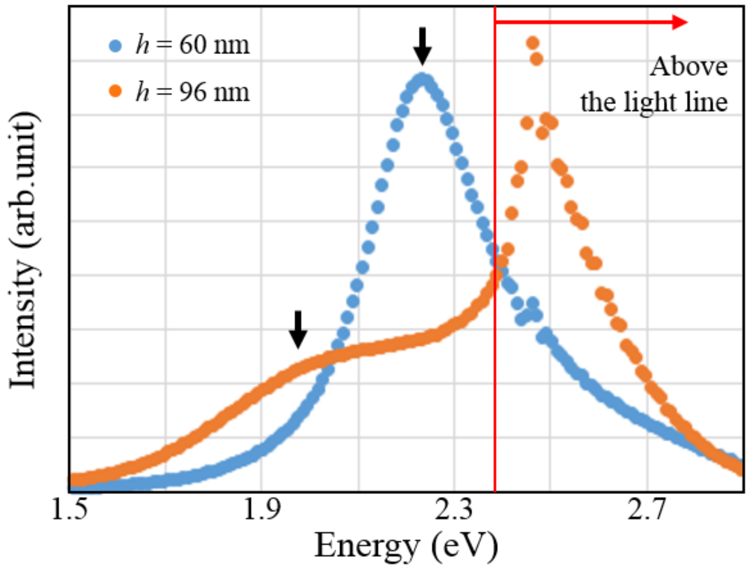


FIG. S4 Emission spectra calculated for the $\mathbf{k}_{\Gamma M2}$ mode with 0.0121 $nm^{-1}$ of wave number. The aqua and orange spectra were calculated on the structures with *h* = 60 nm and *h* = 96 nm, respectively.

***B-4. Localized mode at single disks observed in the spatially-resolved EELS experiment***

As shown in Fig. 1a (main text), there was a peak in the infrared range, which was unexpected since there is no band edge in that energy range. The excited mode was considered to be a radial breathing (RB) mode of single disks since that mode was strongly excited when an electron beam hit the centers of the disks [S6]. However, the wavelength of the lowest order of RB modes should be nearly equal to the diameter of disk, meaning that the modal energy should be in the ultraviolet range if it is excited at the top surface with the diameter of 260 nm.

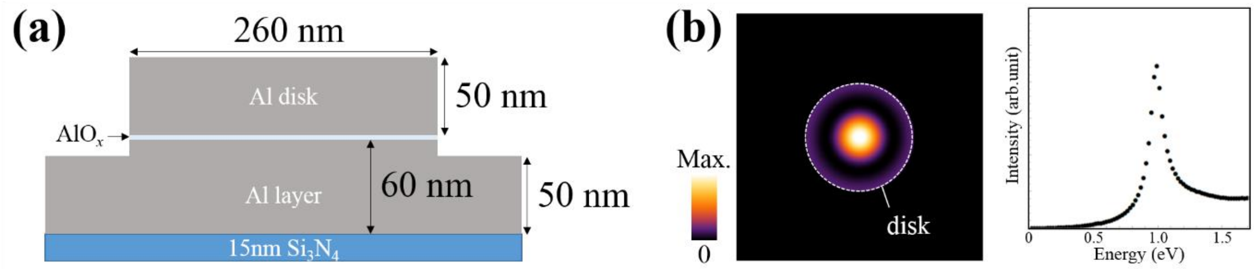


FIG. S5 (a) Model structure with the unexpected oxide layer. (b) Surface normal component of electric field strength of the RB mode in the oxide layer sandwiched by the aluminum layers, and corresponding spectrum. The displayed plane is at the center of the oxide layer.

One possible explanation is the formation of thin oxide layer before the second deposition of aluminum (Fig. S5a). After the first deposition of aluminum for preparation of the aluminum disk array on the $Si_3N_4$ membrane, the sample was taken outside the evaporation chamber for the procedure dissolving the resist layer. As a result, the surface of aluminum disks was exposed in the air. Then, the additional aluminum layer was deposited by 50 nm in thickness. If SPPs can propagate in the oxide layer sandwiched by the aluminum layers, a RB mode can be formed in the infrared range because the wavelength of SPPs is dramatically shorten in gaps sandwiched by metal surfaces [S7]. If the thickness of the oxide layer is assumed to be 3 nm as suggested in literature [S8], the modal energy of RB mode can actually be in the infrared range as shown in the FDTD simulation (Fig. S5b). That calculation was performed on the model structure described in Fig. S5a. The calculation space was set to 600 nm × 600 nm × 328 nm. They were divided by cubic calculation voxels of 1 nm × 1 nm × 1 nm. The sample was placed at the center of calculation space and surrounded in vacuum.

Perfectly matched layers (PMLs) were set at the all sides of the calculation space. The dielectric function for the oxide was set to the constant value 2.62 [S9].

## C. Thickness estimation

The thickness of each deposited aluminum layer was monitored by a quartz oscillator equipped in the evaporation chamber. However, that might have been underestimated as seen in the difference between the measured dispersion relations and the calculation for *h* = 60 nm (Fig. 2d in the main text). The disk height *h* was also estimated from the spatially-resolved EELS data as follows.

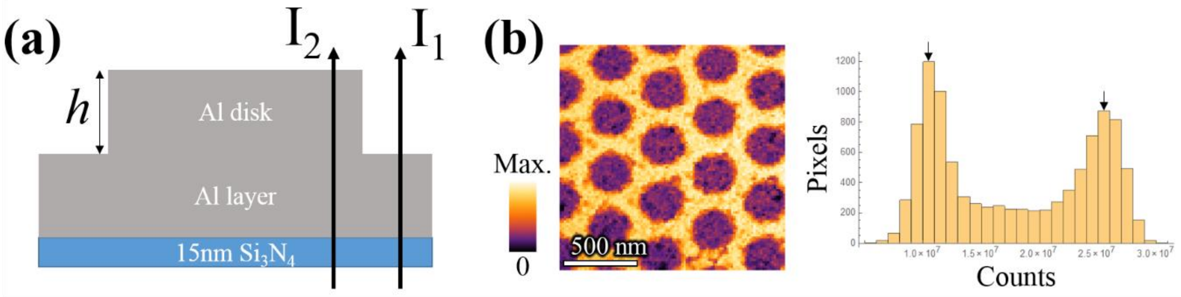


FIG. S6 (a) Two beam paths considered in the thickness estimation. (b) Zero loss peak map taken from the sample (left) and its histogram (right).

The number elastically-scattered electrons at the disks $I_2$ is less than that outside of the disks $I_1$ due to inelastic scattering in the disks. The relationship between $I_1$ and $I_2$ is expressed as follows using the mean free path λ in aluminum,

$$I_2 = I_1 e^{-\lambda h}. \quad \text{(S3)}$$

Fig. S6b shows the zero loss peak map taken from the sample (left) and its histogram (right). There are two peaks in the histogram, which corresponds to $I_1$ and $I_2$. As a result, the disk height *h* was estimated to be 98 nm, which was consistent with the fact that the experimental dispersion relations agreed well with the FDTD calculation for *h* = 96 nm as shown in Fig. 2d in the main text.

**References**


[S1] Palik, E. D. *Handbook of Optical Constants of Solids*. Academic Press, 1998.

[S2] T. Ning, H. Pietarinen, O. Hyvärinen, J. Simonen, G. Genty, and M. Kauranen, Appl. Phys. Lett. **100**, 161902 (2012).

[S3] M. Kociak, and O. Stéphan, Chem. Soc. Rev. **43**, 3865 (2014).

[S4] D. Yoshimoto, H. Saito, S. Hata, Y. Fujiyoshi, and H. Kurata, ACS Photon. **5**, 4476 (2018).

[S5] H. Saito, and N. Yamamoto, Opt. Express **23**, 2524 (2015).

[S6] F.P. Schmidt, A. Losquin, F. Hofer, A. Hohenau, J. R. Krenn, and M. Kociak, ACS Photon. **5**, 861 (2018).

[S7] M. Kuttge, W. Cai, F. J. García de Abajo, and A. Polman, Phys. Rev. B **80**, 033409 (2009).

[S8] H. Saito, K. Namura, M. Suzuki, and H. Kurata, Microscopy **63**, 85 (2014).

[S9] G. Hass, J. Opt. Soc. Am. **39**, 532 (1949).
